# Supplementary material for: General Agentic Memory Via Deep Research
Source: arXiv:2511.18423 source file (2025-11-23)
Supplement: Supplementary file 1 [file appendix.tex]

\section*{Appendix}

\subsection*{Prompts}
